# Supplementary material for: LLM-based Weak Supervision Framework for Query Intent Classification in Video Search
Source: arXiv:2409.08931 source file (2024-09-13)
Supplement: Supplementary file 1 [file Appendix_Persona_Test_Data_Eval.tex]

\begin{table*}[!ht]
\caption{
Test set data evaluation of random persona selection and persona selection via router compared to no persona baseline.}
\vspace{2mm}
\label{tab:persona_test_eval}
\centering
\resizebox{5in}{!}{%
{\footnotesize
\begin{tabular}{@{}cccccccccccc@{}}\toprule
& \multicolumn{3}{c }{\makecell{{Random 3 Personas}}} & \phantom{ab}& \multicolumn{3}{c}{\makecell{{Best 3 Personas via Router}}} \\
\cmidrule{2-4} \cmidrule{6-8}
& \makecell{F1} & \makecell{Precision} & \makecell{Recall} & & \makecell{F1} & \makecell{Precision} & \makecell{Recall}\\  
(Unweighted) \\
\texttt{Claude-v3 Sonnet} & $-4.35\%$ & $-3.36\%$ & $-5.49\%$ && $\textbf{3.27\%}$ & $5.04\%$ & $1.24\%$\\ \\
(Weighted) \\
\texttt{Claude-v3 Sonnet} & $0.81\%$ & $1.37\%$ & $0.20\%$ && $\textbf{3.67\%}$ & $5.67\%$ & $1.51\%$ \\ 
\bottomrule
\end{tabular}
}
}
\end{table*}
