# Supplementary material for: LLM-based Weak Supervision Framework for Query Intent Classification in Video Search
Source: arXiv:2409.08931 source file (2024-09-13)
Supplement: Supplementary file 3 [file appendix_ncd.tex]

\section{A Brief Introduction of the NCD-Based Approach for Text Retrieval}

\label{sec:ncd_approach}
This section explains the NCD-based approach for text retrieval \cite{jiang2023low}. Instead of doing the nearest-neighbor search within the embedding space, this paper propose to search based on the \emph{normalized-compression distance} (NCD), which is written as 
\[
\mathsf{NCD}(X; Y) = \dfrac{C(XY) - \min\left(C(X), C(Y)\right)}{\max\left(C(X), C(Y)\right)}.
\]
Here, $C(\cdot)$ denotes the lengths of the compressed text, and $X$, $Y$ are the input texts (we use gzip as the compressor). Benefits of this method includes $1)$ computational inexpensive as it avoids the encoding stage; and $2)$ comparable performance with the BERT embedding.
